# Supplementary material for: BuildBench: Benchmarking LLM Agents on Compiling Real-World Open-Source Software
Source: arXiv:2509.25248 source file (2026-09-16)
Supplement: Supplementary file 1 [file ICLR_additional_sections.tex]

\newpage
\section*{Reproducibility Statement}
We take measures to ensure the reproducibility of this work. For dataset constructions, we include technical details of raw dataset we sample from and subsequent filtering in Section \ref{sec:dataset_construction}, and the sample size is justified in Section \ref{Sample Size Estimation}. We provide the URLs to access both \href{https://huggingface.co/datasets/STEVENZHANG904/Build_Bench_Test_Data}{test set} and \href{https://huggingface.co/datasets/STEVENZHANG904/Build_Bench_Validation_Data}{validation set} of \datasetname{}. For all experiment implementations, we submit the codebase along with manuscript. 

\section*{Ethics statement}
This work does not raise any ethical concerns and can be conducted without posing risks to individuals, communities, or the broader research environment.
